# Supplementary material for: On Path to Multimodal Generalist: General-Level and General-Bench
Source: arXiv:2505.04620 source file (2025-05-07)
Supplement: Supplementary file 1 [file general-level-5-ranking.tex]

% =============
